# Supplementary material for: Audio Adversarial Examples: Attacks Using Vocal Masks
Source: arXiv:2102.02417 source file (2021-02-06)
Supplement: Supplementary file 1 [file appendix.tex]

\newpage

\appendix
\section*{Appendix}
This Appendix documents our learning points through the process of researching on audio signal separation and writing this paper. Our work relies on open source codes and there are 3 main issues which we will detail in follow subsections in no particular order:
\begin{enumerate}
    \item poor code documentation \label{item:codedocumentation}
    \item compatibility issues, eg. python2 vs python3, pytorch 0.3.0, cuda 8 vs cuda 10 etc. \label{item:codecompatibility}
    \item dependency issues \label{item:depedencyissue}
\end{enumerate}

\section{Initial Problem Formulation} \label{sec:evolution}
Initially, the problem was formulated in a Speech-To-Text solution for noisy audio with concurrent speakers. To be specific, it was a multi-speaker noisy-source separation problem. An example would be YouTube videos. To achieve this, we require four steps:
\begin{enumerate}
    \item \label{item:count1} Count the number of speakers at each time frame
    \item \label{item:count2} Separate out the different speaker signals at each time frame
    \item \label{item:count3} Identify and label every speech time frame with their respective speakers
    \item Perform Speech To Text at each time frame.
\end{enumerate}

\begin{figure*}[h]
  \centering
    \includegraphics[width=1.0\linewidth]{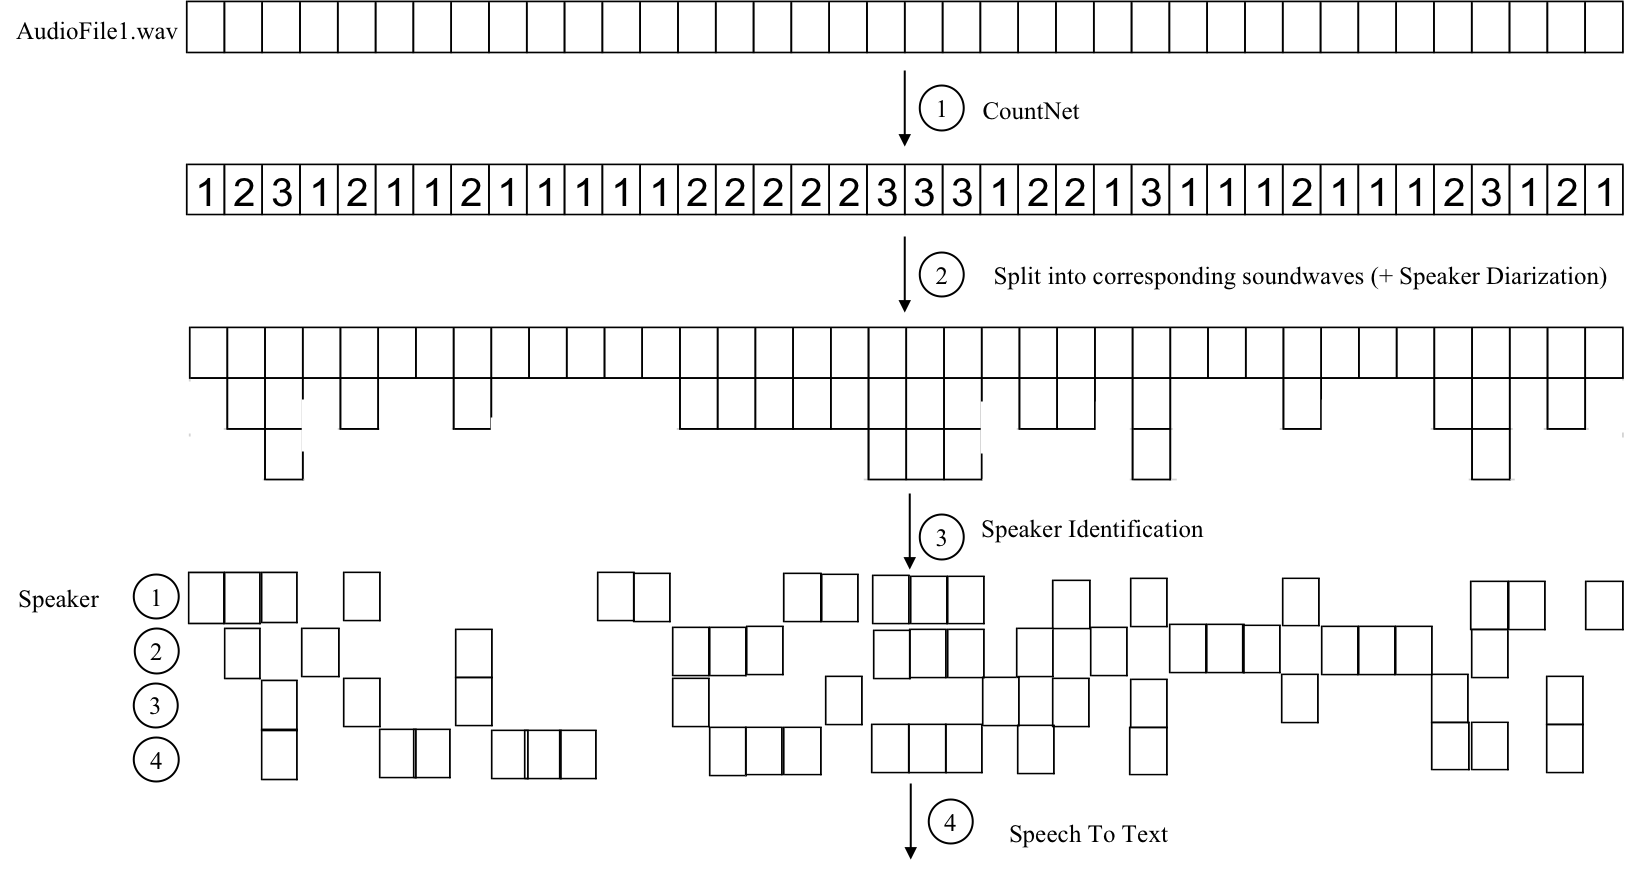}
  \caption{Representation of the Original Problem Formulation}
  \label{fig:originalproblem}
\end{figure*}

The steps are illustrated in Figure \ref{fig:originalproblem}. Several engineers worked on each of the tasks separately. Personnel that worked on (\ref{item:count1}) saw some progress using publicly available repositories, namely CountNet and UIS-RNN. However, personnel that worked on (\ref{item:count2}) faced issues because they were unable to separate the different speaker audio. Although several literature worked on this task, many of these works were not easily reproducible on our part. No personnel worked on (\ref{item:count3}) as it required the output from (\ref{item:count2}). The subsections below documents the challenges we have met, and elaborates on why this initial problem formulation did not materialise.

\subsection{Step 1: Speaker Count} \label{item:step1}

\subsubsection{CountNet}
CountNet \cite{countnet} performs Speaker Count Estimation using deep neural networks. Its code is freely available on Github \cite{countnetCode}. The code uses a recurrent neural network with three Bi-LSTM layers to generate speaker count estimates for 0 to 10 speakers. The model was pre-trained on the LibriSpeech dataset \cite{librispeech}, a corpus based on reading public domain English audio books. 

CountNet counts the number of speakers in a 5 second audio clip. We used the AMI dataset \cite{ami} to perform this experiment. This dataset contains 100 hours of meeting recordings, spoken in English. We break our audio into 2 second clips and pad the audio with silence at the end. This is so that we can have overlapping audio segments to achieve an accurate total number of speakers in the entire audio.

\subsubsection{UIS-RNN}
Unbounded Interleaved-State Recurrent Neural Network (UIS-RNN) \cite{uisrnn} is a work by Google AI Lab. Its code is freely available on Github \cite{uisrnncode}. With an input of an audio file, the work plots the timestamp of each speaker and the number of speakers. The model is trained on the NIST speaker dataset \cite{nist} which contains 148.9 hours of conversational telephone speech. UIS-RNN uses a fully supervised speaker diarization method to count the number of speakers at each time stamp. It models each input speaker by a parameter-sharing RNN using extracted speaker discriminative embeddings from the input audio utterances. This RNN is integrated with a distance-dependent Chinese Restaurant Process to allow for unbounded number of speakers.  

We achieved little success with this library. The output of UIS-RNN is unbounded, hence the number of speakers detected can vary greatly from the ground truth. 

\begin{figure}[h]
  \centering
    \includegraphics[width=1.0\linewidth]{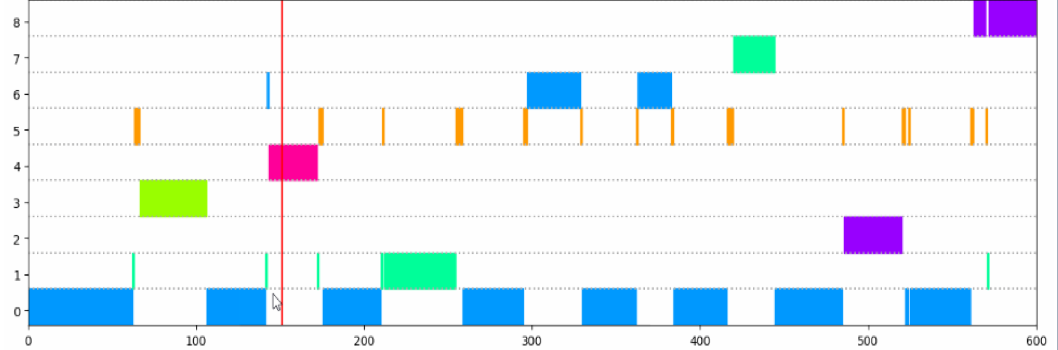}
  \caption{Output of UIS-RNN speaker plot}
  \label{fig:uisrnn}
\end{figure}

\subsection{Step 2: Speaker Separation}

In this step, we utilise speaker count information from \ref{item:step1} in an attempt to separate concurrent speakers.

\subsubsection{uPIT}
Utterance-level Permutation Invariant Training (uPIT) \cite{kolbk2017multitalker} was advertised as a deep-learning based solution to the multi-talker speech separation problem. This work is an extension of their previous work on Permutation Invariant Training (PIT) \cite{yu2016permutation}, which optimises the separation regression error on each iteration of gradient descent, by ignoring the permutation of the mixing of sources. In uPIT, the authors used recurrent neural networks to additionally learn features on utterances, and by minimising the utterance-level separation error, they were successful in separating each speech time frames into their speakers more accurately than PIT.

Thorough experimentation of their uPIT code adapted by other users on github had little success on our part. Our engineers had difficulty in preparing the DARPA-TIMIT dataset into the required \textit{cmvn statistics} for training and inference. 

\subsubsection{Latent Space Visualisation}
We tried visualising two audio inputs in the latent space by running their MFCC outputs through a variational autoencoder (VAE). The idea was to see if projection of the latent points to a higher-dimensional space may serve to separate the speakers if given a single audio input with multiple audio signals.

We plot our results of the projection to 7 dimensional latent space using t-distributed Stochastic Neighbour Embedding (t-SNE).

\begin{figure}[h]
  \centering
  \begin{subfigure}[b]{0.4\linewidth}
    \includegraphics[width=\linewidth]{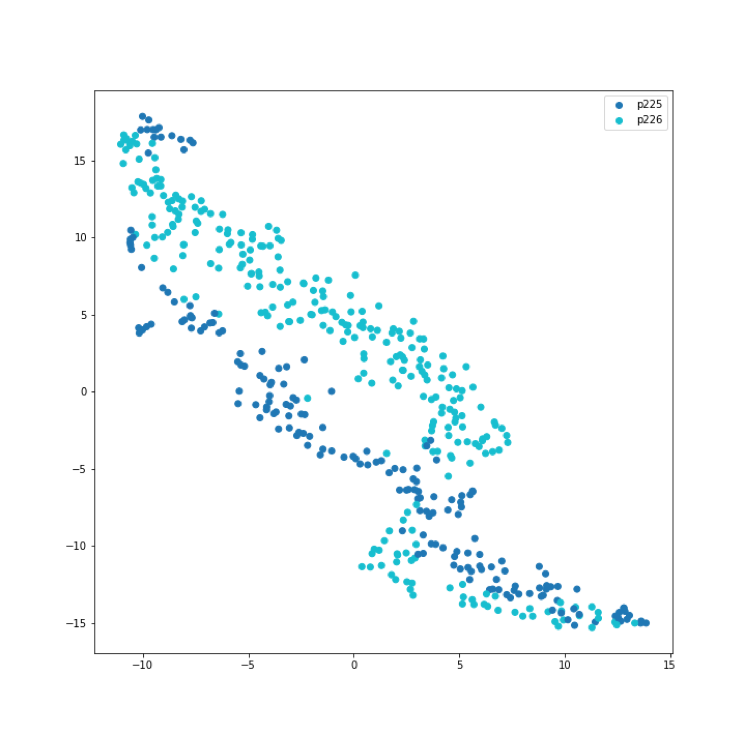}
     \caption{Normalised MFCC Inputs}
  \end{subfigure}
  \begin{subfigure}[b]{0.4\linewidth}
    \includegraphics[width=\linewidth]{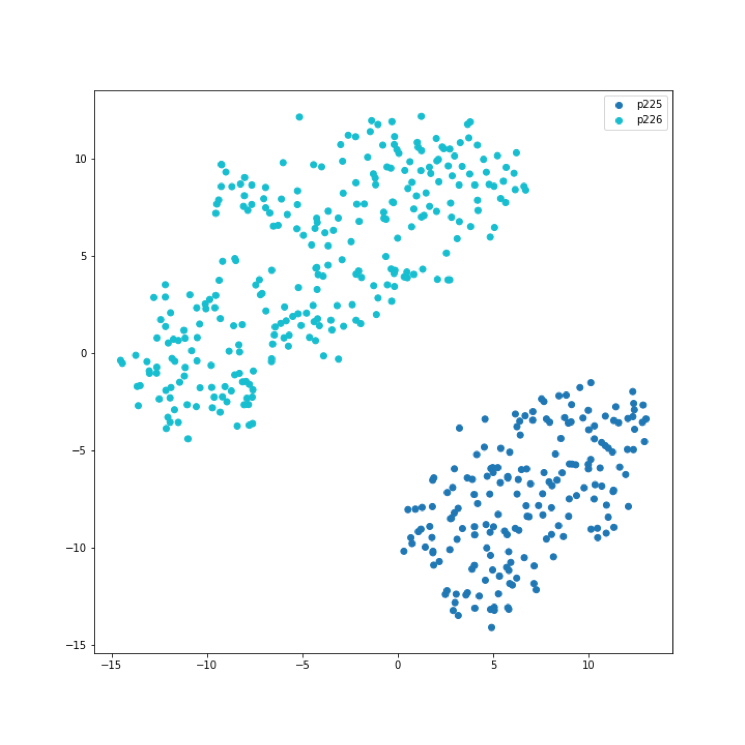}
    \caption{Non-Normalised MFCC Inputs}
  \end{subfigure}
  \caption{7 dimensional latent space plots. Dark blue dots represent the male speaker, light blue dots the female speakers}
  \label{fig:twospeakers}
\end{figure}

\begin{figure}[h]
  \centering
  \begin{subfigure}[b]{0.4\linewidth}
    \includegraphics[width=\linewidth]{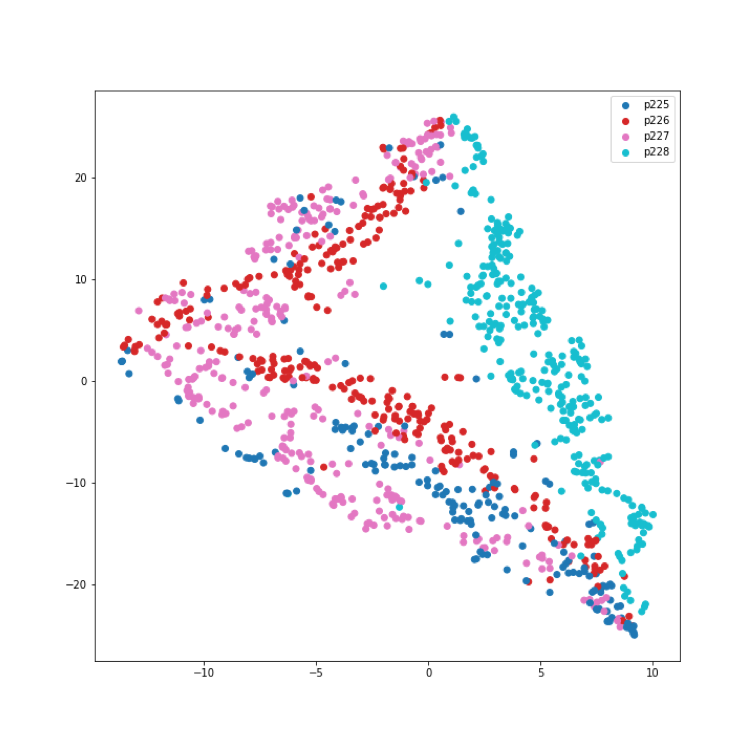}
     \caption{Normalised MFCC Inputs}
  \end{subfigure}
  \begin{subfigure}[b]{0.4\linewidth}
    \includegraphics[width=\linewidth]{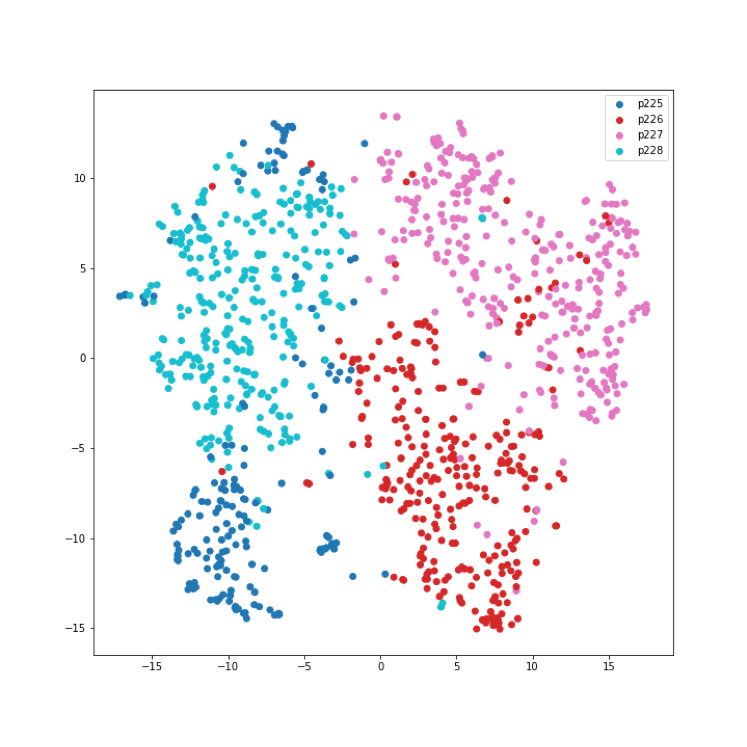}
    \caption{Non-Normalised MFCC Inputs}
  \end{subfigure}
  \caption{7 dimensional latent space plots. Blue dots represent the male speaker, red dots the female speakers}
  \label{fig:fourspeakers}
\end{figure}

Figure \ref{fig:twospeakers} show that it may be possible to separate speakers of different genders, probably because they have different vocal ranges. Non-normalised MFCC inputs provide a better segregation but have a loss value of over 6 digits, while loss values of normalised MFCC inputs are typically in the range of $10^{-2}$. 

We posit that given a single audio file with N number of audio signals, a VAE with N number of sample mean, $\mu$, and sample sigma, $\sigma$, layers will be able to separate the audio signals. However, this dynamic change in a VAE has not been well-explored. This is a possible direction to work towards in the future.

\subsection{Step 3: Speaker Identification}

We posit that with output from (\ref{item:count2}), a typical supervised classification algorithm such as support vector machine (SVM) will be sufficient to classify the output to its respective speakers. However, this would require a labelled dataset.

\subsection{Step 4: Speech To Text}

With the output from (\ref{item:count3}), we posit that a state-of-the-art open sourced automatic speech recognition (ASR) library such as DeepSpeech will be able to transcribe audio from each timeframe into text. A sample resulting output will be the following:

Speaker A (0001-0003): Hi, welcome to this conference call, I am speaker A.

Speaker B (0003-0005): Hi, I am speaker B.

Speaker C (0003-0005): Hi, I am speaker C.

\section{Final Problem Formulation}
We formulated our final problem in response to the difficulties we met in Section \ref{sec:evolution}. As written in the sections before this appendix, utilising properties that caused audio to be inseparable, we worked to generate an audio signal to overlay on an original single source, mono audio channel audio, such that SOTA STT systems are unable to transcribe the audio. The subsections below documents in detail the obstacles we have met while working towards this goal.

\subsection{Wav2Letter++}
Wav2Letter++ \cite{wav2letter} was particularly difficult to install and decode. The documentation on the date of installation was not well written and the number of dependencies required further complicated the issue. We were unable to install some dependency despite the various attempts. Fortunately, wav2letter++ has a working docker image.

Other problems began to surface after installation. The tutorial allowed us to train a model using the LibriSpeech dataset and decode LibriSpeech data, but it was not usable as a decoder for our test set as there was no documentation written for users to prepare a custom test set. However, the wav2letter++ team has provided code recipe for TIMIT. We were able to make use of the recipe to train a model on the TIMIT dataset but this model cannot be used to decode our test set as the given recipe was incomplete:

\begin{enumerate}
    \item the decoding configuration file was missing \label{item:decoding}
    \item there was no documentation on how to prepare lexicons that fit the decoder. \label{item:nodocumentation}
\end{enumerate}

We raised an issue on the above matter at the wav2letter++ github repository and the wav2letter++ team replied in less than a day. Their solution to (\ref{item:decoding}) was to make use of the decoding configuration file from other available recipes such as LibriSpeech but it was not possible as (\ref{item:nodocumentation}) was an issue that needed to be solved for (\ref{item:decoding}) to work. They then proposed to use their pre-trained model, wav2letter@anywhere, for inference purposes, which met our needs. However, we quickly realised that the pre-trained model was buggy and could not run. They resolved the issue within a day and made our final results possible as shown in Table \ref{tab:originalresults}. We are fortunate that the wav2letter++ team is very responsive or we would not have been able to produce results using wav2letter@anywhere.

\subsection{Original Set of Results}
Table \ref{tab:originalresults} presents the full set of results for the experiments in the paper.

\begin{table*}[ht]
\centering
\begin{tabular}{p{2.5cm} p{1.5cm} p{1.5cm} p{1.5cm} p{1.5cm} p{1.5cm} p{1.5cm}}
  \hline
  Audio Files & DeepSpeech & Julius & Kaldi & Wav2letter@ \newline anywhere & CMUSphinx & Humans\\  
  \hline
  $x$                   & 0.13 (0.15) & 0.76 (0.31) & 0.32 (0.20) & 0.16 (0.17) & 0.35 (0.31) & 0.07 (0.10)  \\
  $\delta_0$            & 1.08 (0.20) & 0.99 (0.03) & 1.00 (0.03) & 1.01 (0.13) & 1.29 (0.32) &  -  \\
  $\delta_{-5}$         & 1.08 (0.18) & 1.00 (0.00) & 1.00 (0.03) & 1.01 (0.13) & 1.26 (0.30) &  - \\
  $\delta_{-10}$        & 1.09 (0.23) & 1.00 (0.00) & 1.00 (0.19) & 1.01 (0.13) & 1.23 (0.26) &  - \\
  $\delta_{-15}$        & 1.14 (0.31) & 1.00 (0.00) & 1.01 (0.03) & 1.03 (0.14) & 1.12 (0.23) &  - \\
  $\delta_{-20}$        & 1.06 (0.12) & 1.00 (0.00) & 1.00 (0.00) & 1.02 (0.13) & 1.09 (0.22) &  - \\
  $x + \delta_0$        & 1.03 (0.26) & 0.99 (0.19) & 0.90 (0.18) & 0.87 (0.22) & 1.26 (0.40) & 0.77 (0.36)  \\
  $x + \delta_{-5}$     & 0.82 (0.27) & 0.93 (0.17) & 0.77 (0.22) & 0.65 (0.22) & 1.02 (0.40) &  0.36 (0.30)  \\
  $x + \delta_{-10}$    & 0.63 (0.35) & 0.85 (0.26) & 0.62 (0.27) & 0.42 (0.23) & 0.94 (0.41) &  0.28 (0.29)  \\
  $x + \delta_{-15}$    & 0.35 (0.28) & 0.78 (0.29) & 0.48 (0.28) & 0.26 (0.20) & 0.68 (0.32) & 0.10 (0.11)  \\
  $x + \delta_{-20}$    & 0.23 (0.24) & 0.79 (0.29) & 0.37 (0.23) & 0.18 (0.18) & 0.63 (0.33) & 0.08 (0.11)  \\
  $x + \text{CW}$       & 0.49 (0.31) & 0.84 (0.26) & 0.49 (0.26) & 0.28 (0.25) & 0.85 (0.36) &  0.10 (0.14)  \\
  \hline
\end{tabular}
\caption{Mean (Standard Deviation) WER of transcriptions for our experiments} 
\label{tab:originalresults}
\end{table*}

\section{Other related works}

\subsection{Arabic Speech to Text with Kaldi}
We explored looking at script languages (Arabic) as compared to ascii languages (English). We downloaded broadcast media from the BBC Youtube chaal, the distortion is a negative number, where
smaller values indicate quieter distortions.
While this metric may notnnel and ran them through a transcription model built for Kaldi. This model \cite{arabic} is developed by the Spoken Language Systems Group at MIT and uses an acoustic modelling method to supplement language modelling in transcription and alignment of the speech to text. The model is trained upon the MGB Challenge dataset which contains 1200 hours of Arabic broadcast data from the Aljazeera Arabic TV channel over a span of 10 years. When this model was played on our dataset, we achieved a WER of 34\%.

The data collected for inference was retrieved by using a tool known as youtube-dl \cite{ytdl}. As it was installed using pip3 and the original github repository only had a tutorial for command line flags, we had some issues writing a python program to download audio recordings and their respective transcripts for inference.
